# Supplementary material for: DocStormer: Revitalizing Multi-Degraded Colored Document Images to Pristine PDF
Source: arXiv:2310.17910 source file (2023-10-27)
Supplement: Supplementary file 1 [file X_suppl.tex]

\clearpage
\setcounter{page}{1}
\maketitlesupplementary

\section*{Summary}

\ding{104} We provide in this document supporting materials that cannot fit into the manuscript due to the page limit, including more details of the method pre-analysis, more implementation details of the proposed approaches, and various ablation studies for the experiments in the main manuscript. In particular, we provide here additional results on the fourteen datasets in the main manuscript.

\hspace*{\fill}

\noindent \ding{104} The organizations of this supplementary material are summarized as follows.

\noindent $\blacktriangleright$ \textbf{Sec.~1:} : We begin in Sec. 1 by giving more details and explanations of Method Pre-analysis, corresponding to Sec. 3.3 of the main manuscript.

\noindent $\blacktriangleright$ \textbf{Sec.~2:} Sec. 2: Also, we give in Sec. 2 more descriptions of the various datasets used in the main manuscript and this supplement, mentioned in Sec. 5.1 of the main manuscript.

\noindent $\blacktriangleright$ \textbf{Sec.~3:} Secs. 3, 4, 5, 6, 7, and 8: Furthermore, in the following sections, we provide more implementation details, perform extensive ablation studies including various network architectures and heterogeneous types of GNNs, and demonstrate more visualization results to validate the effectiveness of the proposed series of complementary approaches for GARE.

\section*{Table of Contents}

The table of contents, as well as the lists of figures and tables in this supplementary material are provided below, for the sake of easy reference.

\tableofcontents
\section*{List of Figures}
\listoffigures
\section*{List of Tables}
\listoftables

\sectioin{More visualization about Spatial Attention}
% Your other sections go here. E.g.,
%\section{Method Pre-analysis}
%\section{Datasets}
%...
